# Supplementary material for: Quantization-Aware Imitation-Learning for Resource-Efficient Robotic Control
Source: arXiv:2412.01034 source file (2024-12-02)
Supplement: Supplementary file 1 [file supplement.tex]

\section{QARL+QBC}

\section{Experiments Details}

\subsection{Benchmark Details}

\subsection{Quantization Details}

In this section, we describe the quantization details applied to both the \textit{Roach} and \textit{CILRS} models using the QAIL/QARL methods. For both models, quantization is applied to the image encoder, which constitutes the majority of the computational load, accounting for 97.45\% and 99.9\% of the total FLOPs, respectively. We quantize both weights and activations to 4-bit precision. The quantization of a weight \( w \) is expressed as:
\begin{equation}
\bar{w} = \left\lfloor{\text{clip}\left(\frac{w}{s}, -2^{b-1}, 2^{b-1}-1\right)}\right\rceil, \quad \hat{w} = \bar{w} \cdot s
\end{equation}
where \( s \) is the step size, and \( b \) is the number of bits (for activations, the clip range is from 0 to \( 2^b-1 \)). Following the LSQ~\cite{esser2020learned}, we set the step size as a trainable parameter, allowing it to be learned during training to minimize quantization error.
For backpropagation, we use the Straight-Through Estimator (STE)~\cite{bengio2013estimating} defined as follows:
\begin{equation}
\frac{\partial \hat{w}}{\partial w} = \begin{cases}
1 & \text{if } -2^{b-1} \leq \frac{w}{s} \leq 2^{b-1}-1 \\
0 & \text{otherwise}
\end{cases}
\end{equation}

\section{Visualization}

\section{QARL+QBC}

\subsection{Videos}

\subsection{CILRS}

\begin{itemize}
    \item \textbf{CILRS\_FP.mp4}: An uncut evaluation run recorded in the new-town of the NoCrash-dense benchmark. This video showcases the driving performance of the full-precision \textit{CILRS} model, demonstrating safe driving by slowing down at intersections when other vehicles or pedestrians are present, even if the light is green.
    \item \textbf{CILRS\_QAIL.mp4}: An uncut evaluation run recorded in the new-town of the NoCrash-dense benchmark. This video shows the \textit{CILRS} model with W4A4 QAIL applied, where the vehicle fails to avoid other vehicles at intersections, resulting in collisions.
    \item \textbf{CILRS\_QAIL+QBC.mp4}: An uncut evaluation run recorded in the new-town of the NoCrash-dense benchmark. This video demonstrates the \textit{CILRS} model with W4A4 QAIL+QBC applied, showing safe driving by slowing down at intersections when other vehicles or pedestrians are present, even if the light is green, avoiding collisions.
\end{itemize}

\section{Implementation Details}

For our experimental setup, we utilized NVIDIA's Jetson AGX Orin device, a high-performance system-on-module (SoM) designed for advanced AI and robotics applications. The Jetson AGX Orin is equipped with a 12-core Arm Cortex-A78AE CPU, an NVIDIA Ampere architecture GPU, and 2$\times$ NVDLA v2.0 deep learning accelerators, enabling it to handle complex AI tasks efficiently. The device runs on Ubuntu 20.04 64-bit LTS OS with GNU gcc/g++ version 9.3.0. Additionally, we utilized the 30W power mode on the Jetson AGX Orin.

To measure power consumption in our experiments, we employed the jetson-stats library, which is specifically designed for use with NVIDIA Jetson devices. This library leverages the capabilities of the Triple Channel Voltage/Current Monitor (Texas Instrument INA3221) integrated into Jetson boards. The INA3221 sensor provides detailed measurements of voltage, current, and power consumption for various power rails on the device, allowing for precise monitoring and analysis of the on board power usage.
